# Supplementary material for: Zero-phase-difference Josephson current based on spontaneous symmetry-breaking via parametric excitation of a movable superconducting dot
Source: arXiv:1701.05840 source file (2017-01-20)
Supplement: Supplementary file 1 [file SupplementalMaterial.pdf]

# Supplemental material for "Zero-phase-difference Josephson current based on spontaneous symmetry-breaking via parametric excitation of a movable superconducting dot"

A. M. Eriksson[1] and A. Vikström[1]

[1]Department of Physics, Chalmers University of Technology, Kemigården 1, SE-412 96 Göteborg, Sweden

(Dated: January 20, 2017)

## I. THE DIRECT SUPERCURRENT IN THE LIMIT OF SMALL DEFLECTIONS

Here, we derive an alternate expression for the time-averaged current through the dot and then give an approximate expression which is valid for small mechanical deflections compared to the tunneling length $\lambda$, $\mathrm{Tr}[\hat{x}^2\hat{\rho}] \ll \lambda^2$. As in the main article, we write the time-averaged current as

$$\bar{J} = \frac{1}{T}\int_{-T/2}^{T/2} \mathrm{d}t\ \mathrm{Tr}\left[\hat{J}\hat{\rho}\right], \tag{S1}$$

where $\hat{\rho}$ is the density operator. Here, we write the (Schrödinger picture) current operator in the Josephson representation:

$$\hat{J} = -e\omega_J \sinh\left(\hat{x}/\lambda\right)\hat{\sigma}_y = \frac{-i}{2\hbar}[\hat{H},\hat{q}]\tanh(\hat{x}/\lambda), \tag{S2}$$

with the CPB charge operator $\hat{q} = -e(\hat{I} + \hat{\sigma}_x)$, and the identity and Pauli matrices

$$\hat{I} = \begin{pmatrix}1 & 0\\ 0 & 1\end{pmatrix},\quad \hat{\sigma}_x = \begin{pmatrix}0 & 1\\ 1 & 0\end{pmatrix},\quad \hat{\sigma}_y = \begin{pmatrix}0 & -i\\ i & 0\end{pmatrix},\quad \hat{\sigma}_z = \begin{pmatrix}1 & 0\\ 0 & -1\end{pmatrix}. \tag{S3}$$

We insert eq. (S2) into eq. (S1) and use the cyclic property of the trace to move the commutator to $\hat{\rho}$, allowing us to use the Liouville von-Neumann equation

$$i\hbar\frac{\partial\hat{\rho}}{\partial t} = [\hat{H},\hat{\rho}]. \tag{S4}$$

We then assume the density operator $\hat{\rho}$ to be periodic with period $T = 2\pi/\Omega$ in its stationary state which gives $\int_{-T/2}^{T/2}(\partial_t\hat{\rho})\mathrm{d}t = 0$. Finally we use the relation $[\hat{p}, f(\hat{x})] = -i\hbar f'(\hat{x})$ and arrive at

$$\bar{J} = -\frac{1}{4m\lambda}\frac{1}{T}\int_{-T/2}^{T/2} \mathrm{d}t\ \mathrm{Tr}\left[\left\{\hat{p}, 1 + \tanh^2\left(\frac{\hat{x}}{\lambda}\right)\right\}\hat{q}\hat{\rho}\right], \tag{S5}$$

where $\{\ldots,\ldots\}$ denotes the anticommutator. In the low amplitude regime $\mathrm{Tr}\left[\hat{x}^2\hat{\rho}\right] \ll \lambda^2$, we can approximate the anticommutator by $2\hat{p}$. This results in the final expression for the direct supercurrent in the limit of small deflections,

$$\bar{J} \approx -\frac{1}{T}\int_{-T/2}^{T/2} \mathrm{d}t\ \mathrm{Tr}\left[\frac{\hat{p}}{2m\lambda}\hat{q}\hat{\rho}\right]. \tag{S6}$$

Hence, a finite direct supercurrent requires a time-correlation between the CPB momentum $\hat{p}$ and the CPB charge occupation $\hat{q}$.

## II. TIME-EVOLUTION OF THE ELECTRONIC SUBSYSTEM

The time evolution of the full system is governed by eq. (S4) with the Hamiltonian

$$\hat{H} = \left(\frac{\hat{p}^2}{2m} + \frac{m\omega_m^2\hat{x}^2}{2} + \frac{\eta}{4}\hat{x}^4\right) - \hbar\omega_J\hat{\sigma}_z - \hbar\omega_J\epsilon\cos(\Omega t)\left(\hat{I} + \hat{\sigma}_x\right) - 2\hbar\omega_J\sinh^2\left(\frac{\hat{x}}{2\lambda}\right)\hat{\sigma}_z. \tag{S7}$$

As an approximation, we will disregard quantum entanglement between the mechanical and electronic subsystems and assume that the full density operator of the system can be written as a product state, $\hat{\rho} \approx \hat{\rho}_e \otimes \hat{\rho}_m$, where $\hat{\rho}_e$ ($\hat{\rho}_m$) is the electronic (mechanical) density operator. Since we assume that the amplitude of the mechanical deflection is small, $\mathrm{Tr}\left[\hat{x}^2\hat{\rho}\right] \ll \lambda^2$, we expect that the main influence on the electronic subsystem will be from the ac driving field. We therefore begin by calculating $\hat{\rho}_e$ with the ac driving taken into account but neglecting the electromechanical coupling (the last term in eq. (S7)). The time-evolution operator $\hat{U}(t,0)$ from time 0 to $t$ then fulfills

$$i\hbar\frac{\partial\hat{U}(t,0)}{\partial t} = \left[-\hbar\omega_J\hat{\sigma}_z - \hbar\omega_J\epsilon\cos(\Omega t)\left(\hat{I}+\hat{\sigma}_x\right)\right]\hat{U}(t,0). \tag{S8}$$

To solve this equation we first transform into the interaction picture defined by $\hat{U}(t,0) = \exp(i\hat{\sigma}_z\tilde{\omega}_J t)\tilde{U}(t,0)$ with renormalized frequency $\tilde{\omega}_J = \omega_J(1+[eV_0/(2\hbar\omega_J)]^2)$ which gives

$$i\hbar\frac{\partial\tilde{U}(t,0)}{\partial t} = -eV_0\cos(\Omega t)\Big[\cos(2\tilde{\omega}_J t)\hat{\sigma}_x + \sin(2\tilde{\omega}_J t)\hat{\sigma}_y\Big]\tilde{U}(t,t_0) + \frac{(eV_0)^2}{4\hbar\tilde{\omega}_J}\hat{\sigma}_z\tilde{U}(t,0), \tag{S9}$$

We now seek a perturbative approximation by expanding $\tilde{U}(t,0) \approx 1 + \tilde{U}^{(1)}(t,0) + \tilde{U}^{(2)}(t,0)$ to second order in the small driving parameter $\tilde{\epsilon} = eV_0/(\hbar\tilde{\omega}_J)$. Note that $\tilde{\epsilon} = \epsilon/(1+\epsilon^2/4) = \epsilon + \mathcal{O}(\epsilon^3)$, where $\epsilon = eV_0/\hbar\omega_J$ is the small parameter presented in the main text. We did not mention the technicality of the small discrepancy between $\epsilon$ and $\tilde{\epsilon}$ in the main article for the sake of clarity. We evaluate terms of equal order and find

$$\begin{aligned}
\tilde{U}^{(1)}(t,0) &= \frac{i\tilde{\epsilon}}{2}\Big[f_x(t)\hat{\sigma}_x + f_y(t)\hat{\sigma}_y\Big],\\
\tilde{U}^{(2)}(t,0) &= -\frac{\tilde{\epsilon}^2}{\zeta^+\zeta^-}\left[f_I(t)\hat{I} + if_z(t)\hat{\sigma}_z\right],\\
f_x(t) &= \frac{\sin(\zeta^+\tilde{\omega}_J t)}{\zeta^+} + \frac{\sin(\zeta^-\tilde{\omega}_J t)}{\zeta^-},\\
f_y(t) &= \frac{1-\cos(\zeta^+\tilde{\omega}_J t)}{\zeta^+} + \frac{1-\cos(\zeta^-\tilde{\omega}_J t)}{\zeta^-},\\
f_z(t) &= f_x(t) - \frac{\tilde{\omega}_J\sin(2\Omega t)}{2\Omega},\\
f_I(t) &= f_y(t) - \frac{1-\cos(2\Omega t)}{4},
\end{aligned} \tag{S10}$$

where $\zeta^\pm = 2 \pm \Omega/\tilde{\omega}_J$. Since we are interested in the steady state solution $\hat{\rho}_e^{\mathrm{st}}$, we want to choose the initial condition for $\hat{\rho}_e$ such that we avoid transients in the solution. This can be done by introducing a slow dissipation mechanism which drags the electronic subsystem to equilibrium with an environmental bath with some characteristic time $\tau_e$. According to the $\tau$-relaxation approximation

$$i\hbar\frac{\partial\hat{\rho}_e^{\mathrm{st}}(t)}{\partial t} - \left[\hat{H},\hat{\rho}_e^{\mathrm{st}}\right] = \frac{1}{\tau_e}\left(\hat{\rho}_e^{\mathrm{st}}(t) - \hat{\rho}_{\mathrm{eq}}\right) \tag{S11}$$

with the equilibrium density operator $\hat{\rho}_{\mathrm{eq}} = \exp(-\hbar\omega_J\hat{\sigma}_z/k_BT_b)/\mathrm{Tr}[\exp(-\hbar\omega_J\hat{\sigma}_z/k_BT_b)]$ where $T_b$ is the temperature of the environmental bath. With $\hat{\rho}_e^{\mathrm{st}}(t) = \hat{U}(t,0)\hat{\rho}_e^{\mathrm{st}}(0)\hat{U}^\dagger(t,0)$, the left hand side of eq. (S11) is zero to second order in the small parameter $\tilde{\epsilon}$. Hence, the appropriate choice of initial condition is

$$\hat{\rho}_e^{\mathrm{st}}(0) = \lim_{T'\to\infty}\frac{1}{T'}\int_{-T'/2}^{T'/2} \mathrm{d}t'\hat{U}^\dagger(t',0)\hat{\rho}_{\mathrm{eq}}\hat{U}(t',0) \tag{S12}$$

In the low temperature regime $k_BT_b \ll \hbar\omega_J$, we assume that the electronic equilibrium corresponds to the CPB ground state, $\hat{\rho}_{\mathrm{eq}} = \left(\hat{I}+\hat{\sigma}_z\right)/2$, and get

$$\hat{\rho}_e^{\mathrm{st}}(0) = \frac{1}{2}\hat{I} + \frac{2\tilde{\epsilon}\tilde{\omega}_J^2}{4\tilde{\omega}_J^2 - \Omega^2}\hat{\sigma}_x + \frac{1}{2}\left[1 - \frac{\tilde{\epsilon}^2\tilde{\omega}_J^2(12\tilde{\omega}_J^2 - \Omega^2)}{\left(4\tilde{\omega}_J^2 - \Omega^2\right)^2}\right]\hat{\sigma}_z + \mathcal{O}\left(\epsilon^3\right). \tag{S13}$$

Using the initial condition (S13) and the time-evolution operator (S10), different expectation values can now be calculated. Of special interest is the average charge on the CPB,

$$\mathrm{Tr}\left[\hat{q}\hat{\rho}\right] = -e\mathrm{Tr}\left[(\hat{I}+\hat{\sigma}_x)\hat{\rho}\right] = -e\left[1 + 2\epsilon\cos(\Omega t)\right] + \mathcal{O}\left(\epsilon^3\right) + \mathcal{O}\left(\epsilon^2\frac{\Omega}{\omega_J}\right). \tag{S14}$$

## III. EFFECTIVE MECHANICAL EQUATION FOR PARAMETRIC EXCITATION

In this section we seek an effective equation describing the evolution of the mechanical density operator $\hat{\rho}_m$ when the electronic subsystem is given by $\hat{\rho}_e^{\rm st}$ (derived in section II). We start by inserting the product-state ansatz $\hat{\rho} \approx \hat{\rho}_e \otimes \hat{\rho}_m$ into the Liouville von-Neumann eq. (S4) with the Hamiltonian in eq. (S7). We insert $\hat{\rho}_e^{\rm st}(t) = \tilde{U}^\dagger(t,0)\hat{\rho}_e^{\rm st}(0)\tilde{U}(t,0)$ as given by eqs. (S13) and (S10) and then trace out the electronic subsystem to get an equation for $\hat{\rho}_m = {\rm Tr}_{\rm el}\left[\hat{\rho}\right]$,

$$i\hbar\frac{\partial\hat{\rho}_m}{\partial t} = \left[\frac{\hat{p}^2}{2m} + \frac{m\omega_m^2\hat{x}^2}{2} + \frac{\eta}{4}\hat{x}^4 - 2\hbar\omega_J\sinh^2\left(\frac{\hat{x}}{2\lambda}\right){\rm Tr}_{\rm el}\left[\hat{\sigma}_z\hat{\rho}_e^{\rm st}\right], \hat{\rho}_m\right]. \tag{S15}$$

We see that the electronic subsystem generates an effective force on the mechanical subsystem via the electromechanical coupling. Using the results of section II, the force is proportional to

$${\rm Tr}_{\rm el}\left[\hat{\sigma}_z\hat{\rho}_e^{\rm st}\right] = 1 + \epsilon^2\frac{1}{2}\left[1 - \frac{1}{2}\cos\Big(2\Omega t\Big)\right] + \mathcal{O}\left(\epsilon^3\right) + \mathcal{O}\left(\epsilon^2\frac{\Omega}{\omega_J}\right). \tag{S16}$$

Again, we assume small mechanical deflections compared to the tunneling length and expand the force to second order in $a_0/\lambda$ with zero-point amplitude of fluctuations $a_0 = \sqrt{\hbar/(2m\omega_m)}$. We thereby arrive at an effective equation

$$i\hbar\frac{\partial\hat{\rho}_m}{\partial t} = \left[\frac{\hat{p}^2}{2m} + \frac{m\tilde{\omega}_m^2\hat{x}^2}{2} + \frac{\eta}{4}\hat{x}^4 + \epsilon^2\frac{\hbar\omega_J}{8\lambda^2}\hat{x}^2\cos(2\Omega t), \hat{\rho}_m\right]. \tag{S17}$$

with renormalized mechanical frequency $\tilde{\omega}_m^2 = \omega_m^2 - \hbar\omega_J/(m\lambda^2)$. This describes a parametrically driven anharmonic quantum oscillator.

## IV. SEMI-CLASSICAL DIRECT SUPERCURRENT

The semi-classical counterpart to the expression for the direct supercurrent, eq. (S1), is obtained by assuming that we can make the replacement $\hat{x} \to x$. Again, assume small deflections and approximate to second order, $\tanh(x/\lambda) \approx x/\lambda$. Then we use the Liouville von-Neumann equation for the electronic subsystem and integrate by parts. We arrive at an expression for the semi-classical direct supercurrent,

$$\bar{J}_{\rm cl} \approx -\frac{1}{2\lambda T}\int_{-T/2}^{T/2} {\rm d}t\; \dot{x}(t){\rm Tr}\left[\hat{q}\hat{\rho}\right]. \tag{S18}$$

This expression could have been obtained directly from eq. (S6) by the semi-classical assumption, $\hat{p} \to m\dot{x}$. We see that to have a direct supercurrent, there must be a time-correlation between the velocity of the CPB and its charge. In the semi-classical case we have the same time evolution for the electronic subsystem as we have in the quantum case (section II) since we do not take into account the coupling to the mechanics. Thus, the steady-state $\hat{\rho}_e^{\rm st}$ of the electronic subsystem is known and the expectation value of the charge is given by eq. S14. We will now use the semi-classical approach to find stationary solutions for the CPB velocity.

The semi-classical equation for the mechanical deflection is

$$\ddot{x} + \gamma\dot{x} + \omega_m^2 x + \eta x^3 = \xi(t) - \frac{1}{m}\frac{\partial}{\partial x}{\rm Tr}\left[\hat{H}_{\rm J}(x)\rho\right], \tag{S19}$$

where $\gamma$ is a small damping coefficient, $\eta$ corresponds to a weak nonlinearity, $\xi(t)$ is a stochastic force due to interaction with the environment, and the last term describes an effective force from the electronic subsystem due to the electromechanical coupling.

The equation is simplified by inserting eq. (S16) and introducing scaled time $\tau = \tilde{\omega}_m t$, position $X = x/a_0$, damping $\gamma_0 = \gamma/\tilde{\omega}_m$ and nonlinearity $\eta_0 = \eta a_0^2/\tilde{\omega}_m^2$, which gives

$$\ddot{X} + \Big(1 + \delta\cos\left[2(1+\Delta)\tau\right]\Big)X = -\gamma_0\dot{X} - \eta_0 X^3 \tag{S20}$$

with the effective driving strength parameter

$$\delta = \frac{1}{2}\epsilon^2\frac{\omega_J}{\tilde{\omega}_m}\left(\frac{a_0}{\lambda}\right)^2 \tag{S21}$$

and detuning

$$\Delta = \frac{\Omega - \tilde{\omega}_m}{\tilde{\omega}_m} \ll 1. \tag{S22}$$

Eq. (S20) describes the well known parametrically excitable, damped, anharmonic oscillator.[1] To begin with, we disregard the stochastic force $\xi(t)$. We then seek a stationary solution for $X$ using the ansatz

$$X(\tau) = \sqrt{2E(\tau)}\cos[(1 + \Delta/2)\tau + \varphi(\tau)] \tag{S23}$$

with slowly time-varying amplitude squared $E \geq 0$ and phase $-\pi \leq \varphi < \pi$. Of course, we could also use a representation similar to the one in the main article where we use two amplitudes for the $\sin(\Omega t)$ and $\cos(\Omega t)$ terms. However, the energy-phase representation in eq. (S23) clearly shows the phase of the two mechanical states which is convenient when considering phase-flipping processes later on. Following the reasoning by Landau and Lifshitz,[1] we use the compatibility relation to accurately account for resonant terms and get to first order accuracy in the small parameters $\Delta$, $\gamma_0$ and $\eta_0$ the equations

$$\dot{E} = \frac{1}{2}E(\delta \sin(2\varphi) - 2\gamma_0), \tag{S24}$$

$$\dot{\varphi} = \frac{1}{4}(\delta \cos(2\varphi) - 2\Delta + 3\eta_0 E). \tag{S25}$$

The zero-amplitude state $E = 0$ is unstable if

$$\delta^2 > 4(\gamma_0^2 + \Delta^2). \tag{S26}$$

Eq. (S26) will be referred to as the excitation criterion, and the parameter region in which it is fulfilled will be referred to as the excitation region. In the excitation region there are two linearly stable solutions (labeled by $\pm$):

$$E^*_\pm = \frac{1}{3\eta_0}\left(\sqrt{\delta^2 - 4\gamma_0^2} + 2\Delta\right) \equiv E^*, \tag{S27}$$
$$\varphi^*_\pm = \pi\left(1 \pm \frac{1}{2}\right) - \frac{1}{2}\arcsin\left(\frac{2\gamma_0}{\delta}\right).$$

The two stable solutions have equal amplitude $E^*$ but a phase difference of $\pi$. The initial conditions determine which of the two solutions the system will approach. We recognize these two stable solutions as the semi-classical counterparts to the mechanical components of the chiral states we introduced in the quantum-mechanical calculation.

To calculate the semi-classical direct supercurrent eq. (S1), we use eq. (S27) with eq. (S14) and obtain

$$\bar{J}^\pm_{\text{cl}} \approx \pm e\Omega \frac{a_0\sqrt{2E^*}}{\lambda}\frac{eV_0}{2\hbar\omega_J}. \tag{S28}$$

in the two semi-classical states. Recognizing $a_0\sqrt{2E^*}$ as the mechanical amplitude, we see that this is in agreement with the expression we get from the quantum approach (eq. (9) in the main article).

[1] L. Landau and E. Lifshitz, *Mechanics*, Butterworth-Heinemann (Butterworth-Heinemann, 1976), ISBN 9780750628969, URL https://books.google.se/books?id=e-xASAehg1sC.
